# Supplementary material for: A yeast cell cycle pulse generator model shows consistency with multiple oscillatory and checkpoint mutant datasets
Source: arXiv:2302.12946 source file (2023-02-25)
Supplement: Supplementary file 1 [file Supplement.tex]

\begin{figure}[!h]
\centering
\includegraphics[width=.8\textwidth]{wt_clb2_poset_.1.pdf}
\caption{The poset corresponding to a 10\% noise level for wild-type data. \Julian{fix}}
\label{fig:orlando_poset_.1}
\end{figure}
We will now reference Figure \ref{fig:orlando_poset_.1} for a description of the properties of the poset of extrema created within DSGRN. Here we have a constructed a poset of extrema for a time series data set from a replicate of the wild-type yeast cell present in \cite{orlando:2008}.  Through inspection of Figure \ref{fig:orlando_poset_.1} we can see which extrema are comparable and which are incomparable. For example, the node NDD1 min on the top row of the graph is comparable with the node NDD1 max and YHP1 max in the second row but incomparable with Clb2 min, Swi5 min, or Swi4 max also in the second row. This means that within the given noise level NDD1 min is disjoint from NDD1 max and YHP1 max yet not disjoint from Clb2 min, Swi5 min, or Swi4 max. As an example of a total order corresponding to the poset in Figure \ref{fig:orlando_poset_.1}, notice that there exists a path from node Yhp1 min in the top row to Swi5 
max in the bottom row. There actually exists multiple linear extensions, or total orders, to get from Yhp1 min to Swi5 max. The first example being Yhp1 min to Swi5 max in the third row to NDD1 max in the fourth row to Swi5 max in the bottom row. Another example for a total order would be Yhp1 min to Yhp1 max in the second row to Swi5 min in the fourth row to Swi5 max in the bottom row.
